# Supplementary material for: Exploiting symmetries in nuclear Hamiltonians for ground state preparation
Source: arXiv:2402.10277 source file (2024-02-15)
Supplement: Supplementary file 1 [file supplementary.tex]

\appendix

\setcounter{page}{1}

\setcounter{figure}{0} 

\onecolumngrid

\begin{center}
\large{ Supplementary Material for \\ ``Exploiting Symmetries in Nuclear Hamiltonians for Improved Trainability''
}
\end{center}

\section{XXX}
%\label{sct:generalization-bounds-prelims}

\clearpage
